# Supplementary material for: Simultaneous Modeling of Multiple Complications for Risk Profiling in Diabetes Care
Source: arXiv:1802.06476 source file (2018-02-19)
Supplement: Supplementary file 1 [file appendix.tex]

\appendix
%Appendix A
\section{Parameter Estimation}

We summarize the parameter estimation procedure in Algorithm \ref{alg:Estimation}.

\begin{algorithm}%[!t] 
\DontPrintSemicolon 
\KwIn{Observations $\mathcal D = \{x_i, c_{ki}\}$, hyperparameters $\Phi=\{\mathbf\Omega_0, \delta, \nu\}$, learning rate $\epsilon $.} 
\KwOut{Estimated $\hat{\Theta} = \left\{\{\WW_z, \mathbf{\Sigma}_z\}_{z=1}^Z, \mathbf{\Omega}, \UU, \tau\right\}$} 
\Begin{
Initialize $\Theta$ \;
\Repeat{convergence or reach max\_iter}{
    \tcp{Update $\WW$ and $\UU$ using SGD}
    \For{each $k \in \{1,\cdots, K\}$ }{
        Given an instance $\langle x_i, c_{ki}\rangle$ \;
        \For{each $z \in \{1,\cdots, Z\}$ }{
            $ \ww_k^{\mathcal G_z} \leftarrow \ww_k^{\mathcal G_z} - \epsilon  \frac{\partial \mathcal O }{\partial \ww_k^{\mathcal G_z}} $ (Equation (\ref{update_Wz}))\;
        }
        $ \uu_k \leftarrow \uu_k - \epsilon  \frac{\partial \mathcal O }{\partial \uu_k} $ (Equation (\ref{update_u}))\;
    }
    Update $\tau$ by $ \tau \leftarrow \tau - \epsilon  \frac{\partial \mathcal O }{\partial \tau} $ (Equation (\ref{update_lambda}))\;
    Update $\mathbf\Omega$  according to Equation (\ref{update_Omega}) \;
    \For{each $z \in \{1,\cdots, Z\}$ }{
        Update $\mathbf{\Sigma}_z$ according to Equation (\ref{update_Sigma}) \;
    }
}
\Return $\hat{\Theta}$\;
} 
\caption{Parameter Estimation} 
\label{alg:Estimation}
\end{algorithm}
